# Supplementary material for: NormalCrafter: Learning Temporally Consistent Normals from Video Diffusion Priors
Source: arXiv:2504.11427 source file (2025-04-15)
Supplement: Supplementary file 1 [file X_suppl.tex]

\clearpage
\setcounter{page}{1}
\maketitlesupplementary

\setcounter{section}{0}

In this supplementary, we first elaborate implementation details in~\cref{supp:detials}.
Then, we show more qualitative comparison in~\cref{supp:ablation} and~\cref{supp:sample}.

\section{More Details about Implementation}
\label{supp:detials}
\textbf{Data Resampling.}
Since our maximum number of frames is 14, we further divide long videos into shorter clips to ensure balanced sampling during training.
For hypersim, after obtaining 613 videos, we segment them into 1,780 shot clips, each containing between 30 and 60 frames. In order to get a comparable number of samples with single-image datasets. We upsample 1,780 clips 40 times and get 71,200 clips.
For MatrixCity, we divide the 2,316 videos to 7601 short clips and then upsample 10 times, yielding 76010 clips.
For Replica, 3D Ken Burns and Objaverse, we do not resample.

\textbf{Augmentation.} 
During training, the input image goes through the following set of data augmentation ($p$: the probability of applying each augmentation).
\begin{itemize}
    \item \textbf{Random Horizontal Flipping} ($p$ = 0.5). Horizontally flip the clips.
    \item \textbf{Random Croping} ($p = 0.3$). Crop the image with varying aspect ratios.
    \item \textbf{Color} ($p = 0.1$). Distort the color of input clips by changing brightness, contrast, saturate and hue.
    \item \textbf{Grayscale} ($p = 0.2$). Change the image into grayscale.
\end{itemize}
Note, \textbf{Random Croping}, \textbf{Color} and \textbf{Grayscale} are mutually exclusive.

\section{Effectiveness of the Two-stage Training Strategy}
\label{supp:ablation}
In ``\textbf{index.html}", we show more qualitative comparison of \textbf{Ours w/o Stage1} and \textbf{Ours}.

\section{More Results}
\label{supp:sample}
In ``\textbf{index.html}", we show more qualitative with \textbf{StableNormal} and \textbf{Marigold-E2E-FT} on the DAVIS dataset and Sora-generated videos.
